# Supplementary material for: Coarse Correspondences Boost Spatial-Temporal Reasoning in Multimodal Language Model
Source: arXiv:2408.00754 source file (2024-11-21)
Supplement: Supplementary file 1 [file 99-supp.tex]

\appendix

\section*{Appendix}
\section{Broader Impact}
Our method aims at improving the trustworthiness and reliability of deployment of MLLMs in real world application, including but not limited to Vision Pro, autonomous driving, and also humanoid robots. To have a virtual assistant like JARVIS in Marvel films, it's necassry to align the understanding of vision-language model with human's understanding, so that we can ensure safe application of these applications. 
Further, we are committed to reducing the carbon emissions produced by these models. By employing our coarse correspondence prompting method, we use a much smaller tracking module to reduce the number of input used as input to large GPT model. Besides, we also improve the speed and lower the cost of calling OpenAI API to understand a 3d scene. This enables democratize MLLMs so that more people and small companies can create their own real-world applications based on GPT-4V. We hope our work can make large AI models more effectively used for social good.

Still, we would like to point out that with the development of MLLMs, increased reliance on advanced MLLMs could also lead to a reduction in human skills, especially in interpreting and interacting with visual content. Over-dependence on these models might erode critical thinking and analytical abilities in the long term.

\section{More Discussions}
\noindent \textbf{Relation to SlowFast}
SlowFast~\cite{feichtenhofer2019slowfast} is a framework for video recognition that includes two parallel pathways: a Slow pathway that captures motion information at a high frame rate and a Fast pathway that captures semantic information at a low frame rate. The information from both pathways is fused through lateral connections for downstream video recognition tasks.
In a way, our coarse correspondence prompting can be seen as another form of SlowFast. However, unlike SlowFast, where the Slow and Fast pathways operate in parallel, our framework operates sequentially. First, it captures low-level, class-agnostic motion information at a high frame rate using a lightweight tracking model. Then, at a low frame rate, it performs recognition and reasoning requiring semantic understanding using larger MLLMs. The two stages are bridged through visual prompting.
Moreover, while SlowFast learns a representation of the input video for pure vision recognition tasks such as action classification and detection, our coarse correspondence framework aims to better understand the 3D spatial structure and temporal information contained in the input video to achieve spatiotemporal perception and reasoning simultaneously.

\noindent \textbf{Eulerian vs Lagrangian} If deep learning-based methods represent camera or object motion in videos from an Eulerian viewpoint—i.e., expressing how features at fixed locations evolve over time through a multi-dimensional tensor—then our framework adds a Lagrangian viewpoint to this representation. The Lagrangian viewpoint describes the trajectories of entities moving through space and time in the video. Previously, the Lagrangian viewpoint in video descriptions has been shown to better aid human action recognition~\cite{rajasegaran2023benefits}. Here, we demonstrate that it can more generally help 
MLLMs understand the 4D spatiotemporal context represented in videos.

\section{Qualitative Case Study}

\begin{figure}[]
    \centering
    \begin{subfigure}{0.49\textwidth}
        \centering
        \includegraphics[width=1\linewidth]{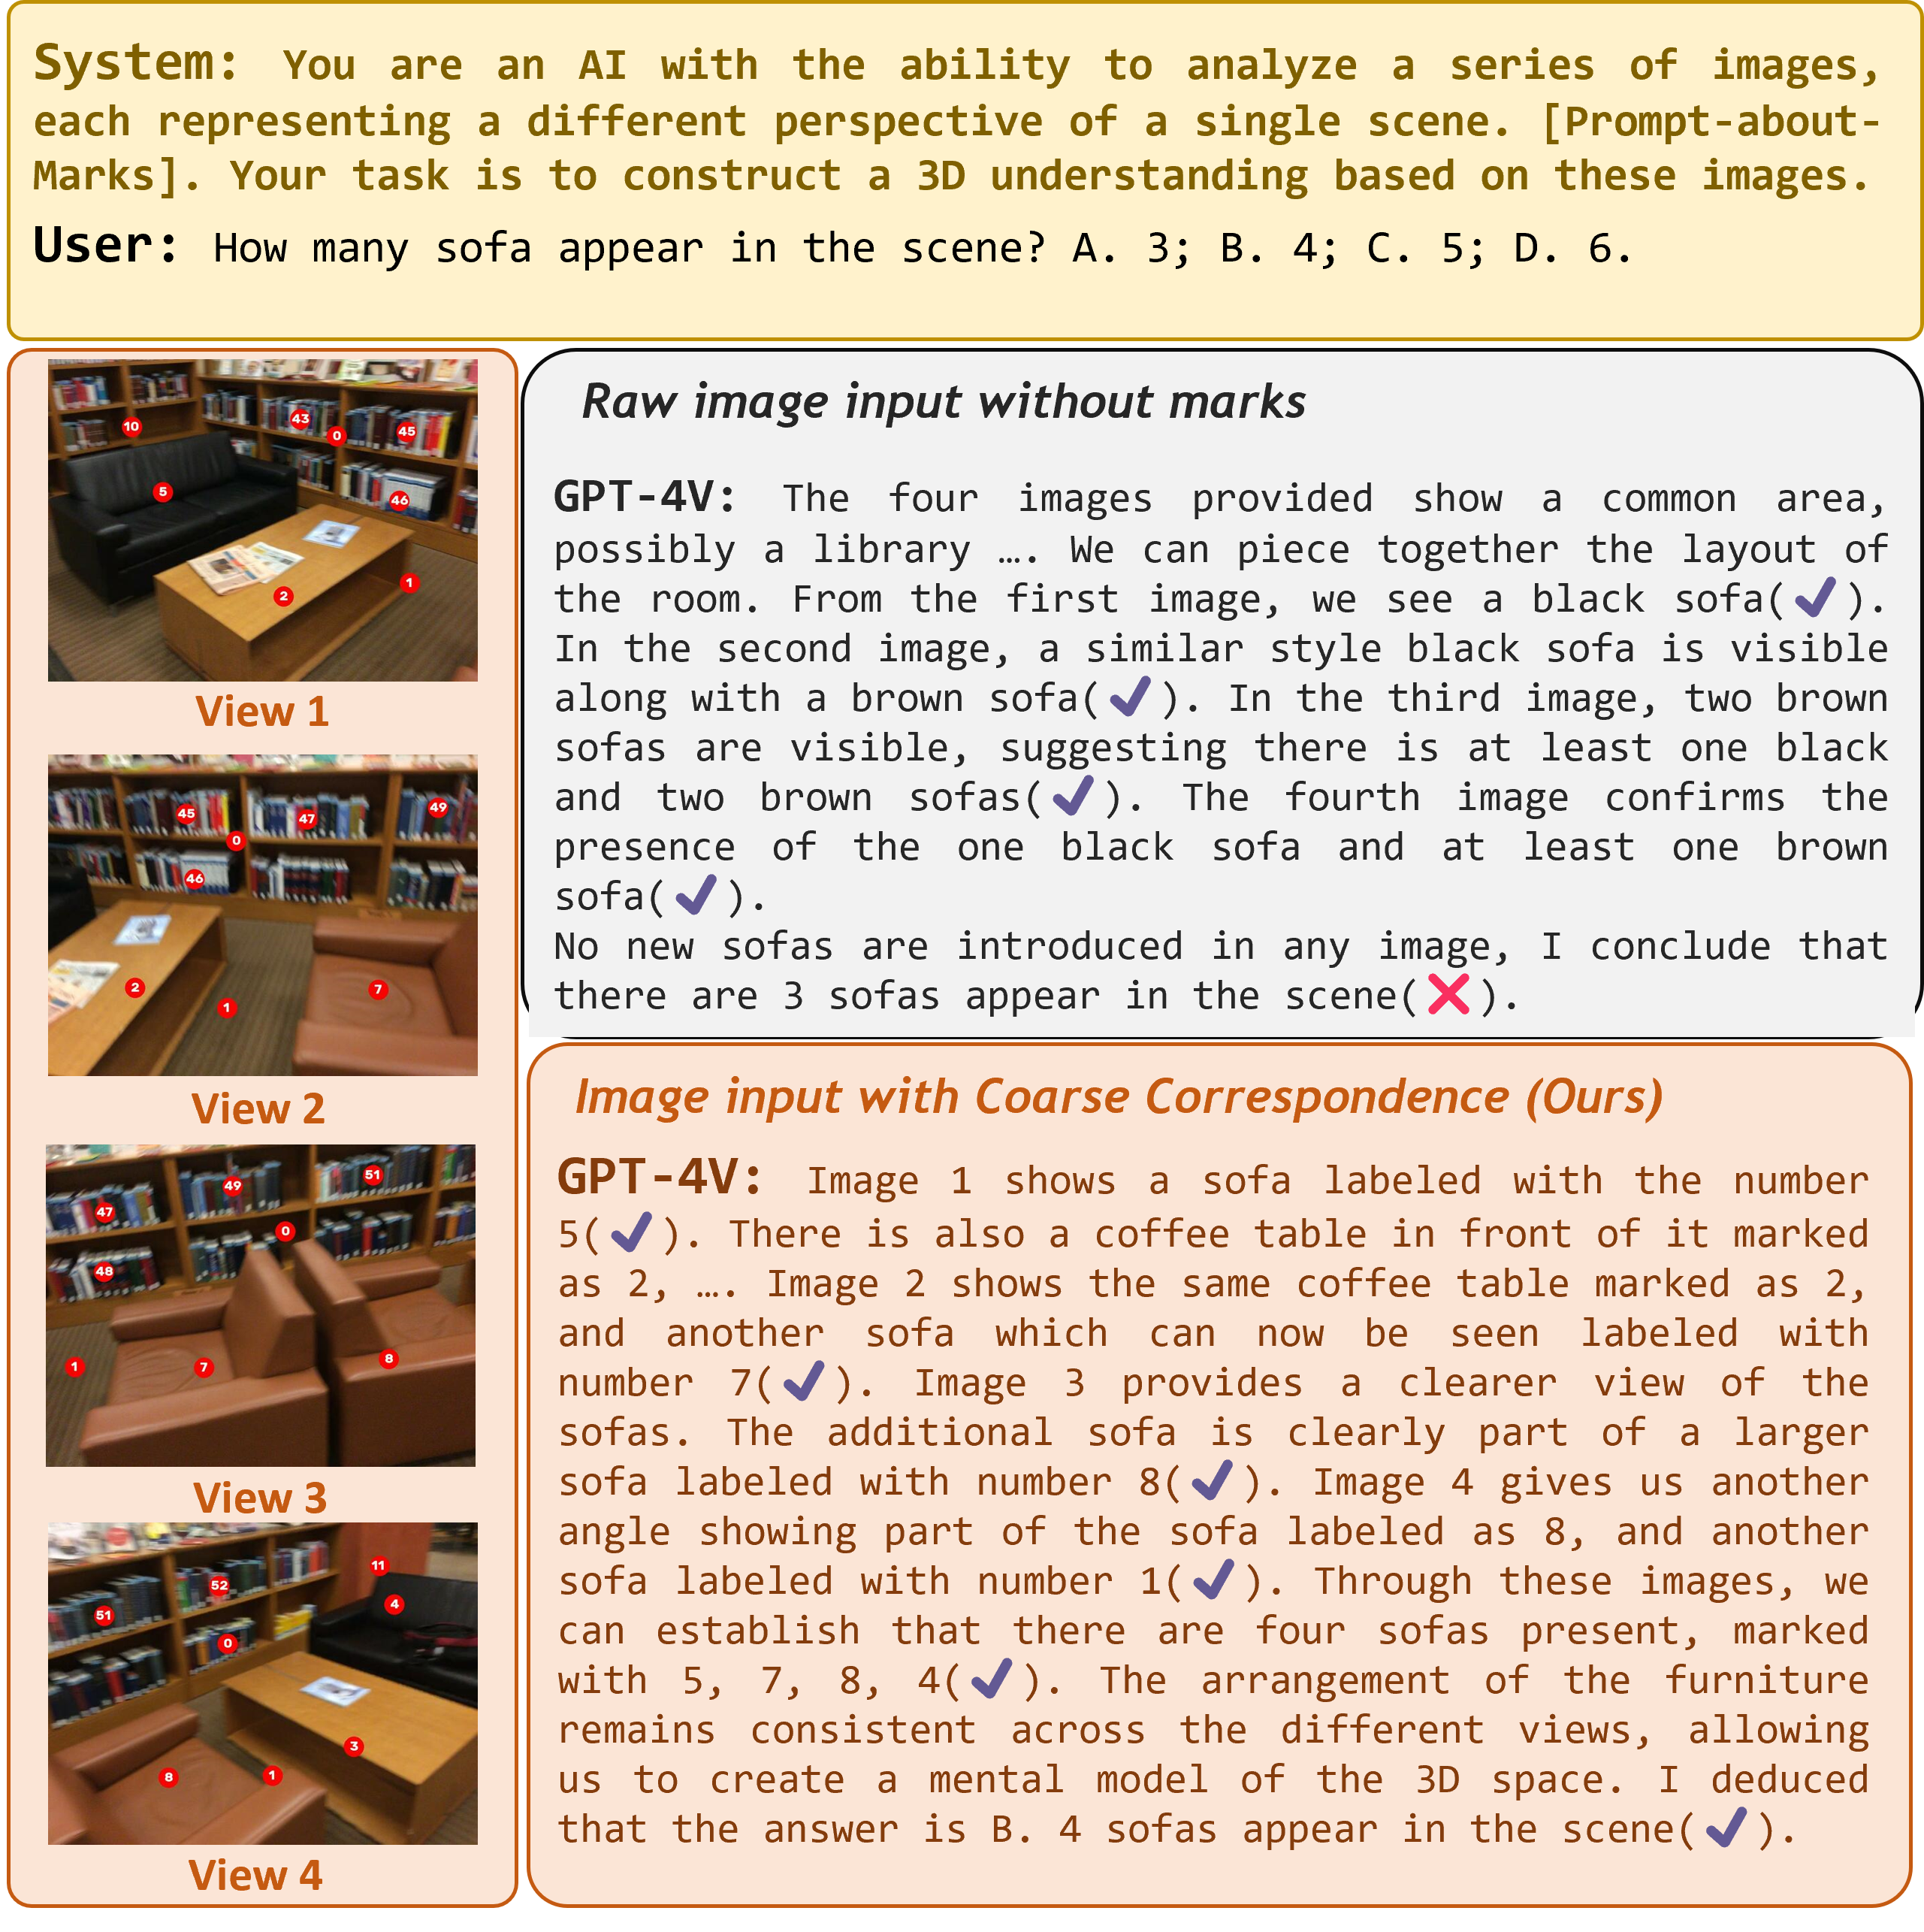}
        \caption{\textbf{Task: Duplicate Objects Counting.} There are 2 brown sofas and 2 black sofas. The brown sofas in View 2\&4 are duplication of those in View 3. Only with the help of the Coarse Correspondence can GPT-4V understand duplicate objects between different views across a single 3D scene.}
        \label{fig:counting}
    \end{subfigure}\hfill
    \begin{subfigure}{0.49\textwidth}
        \centering
        \includegraphics[width=1\linewidth]{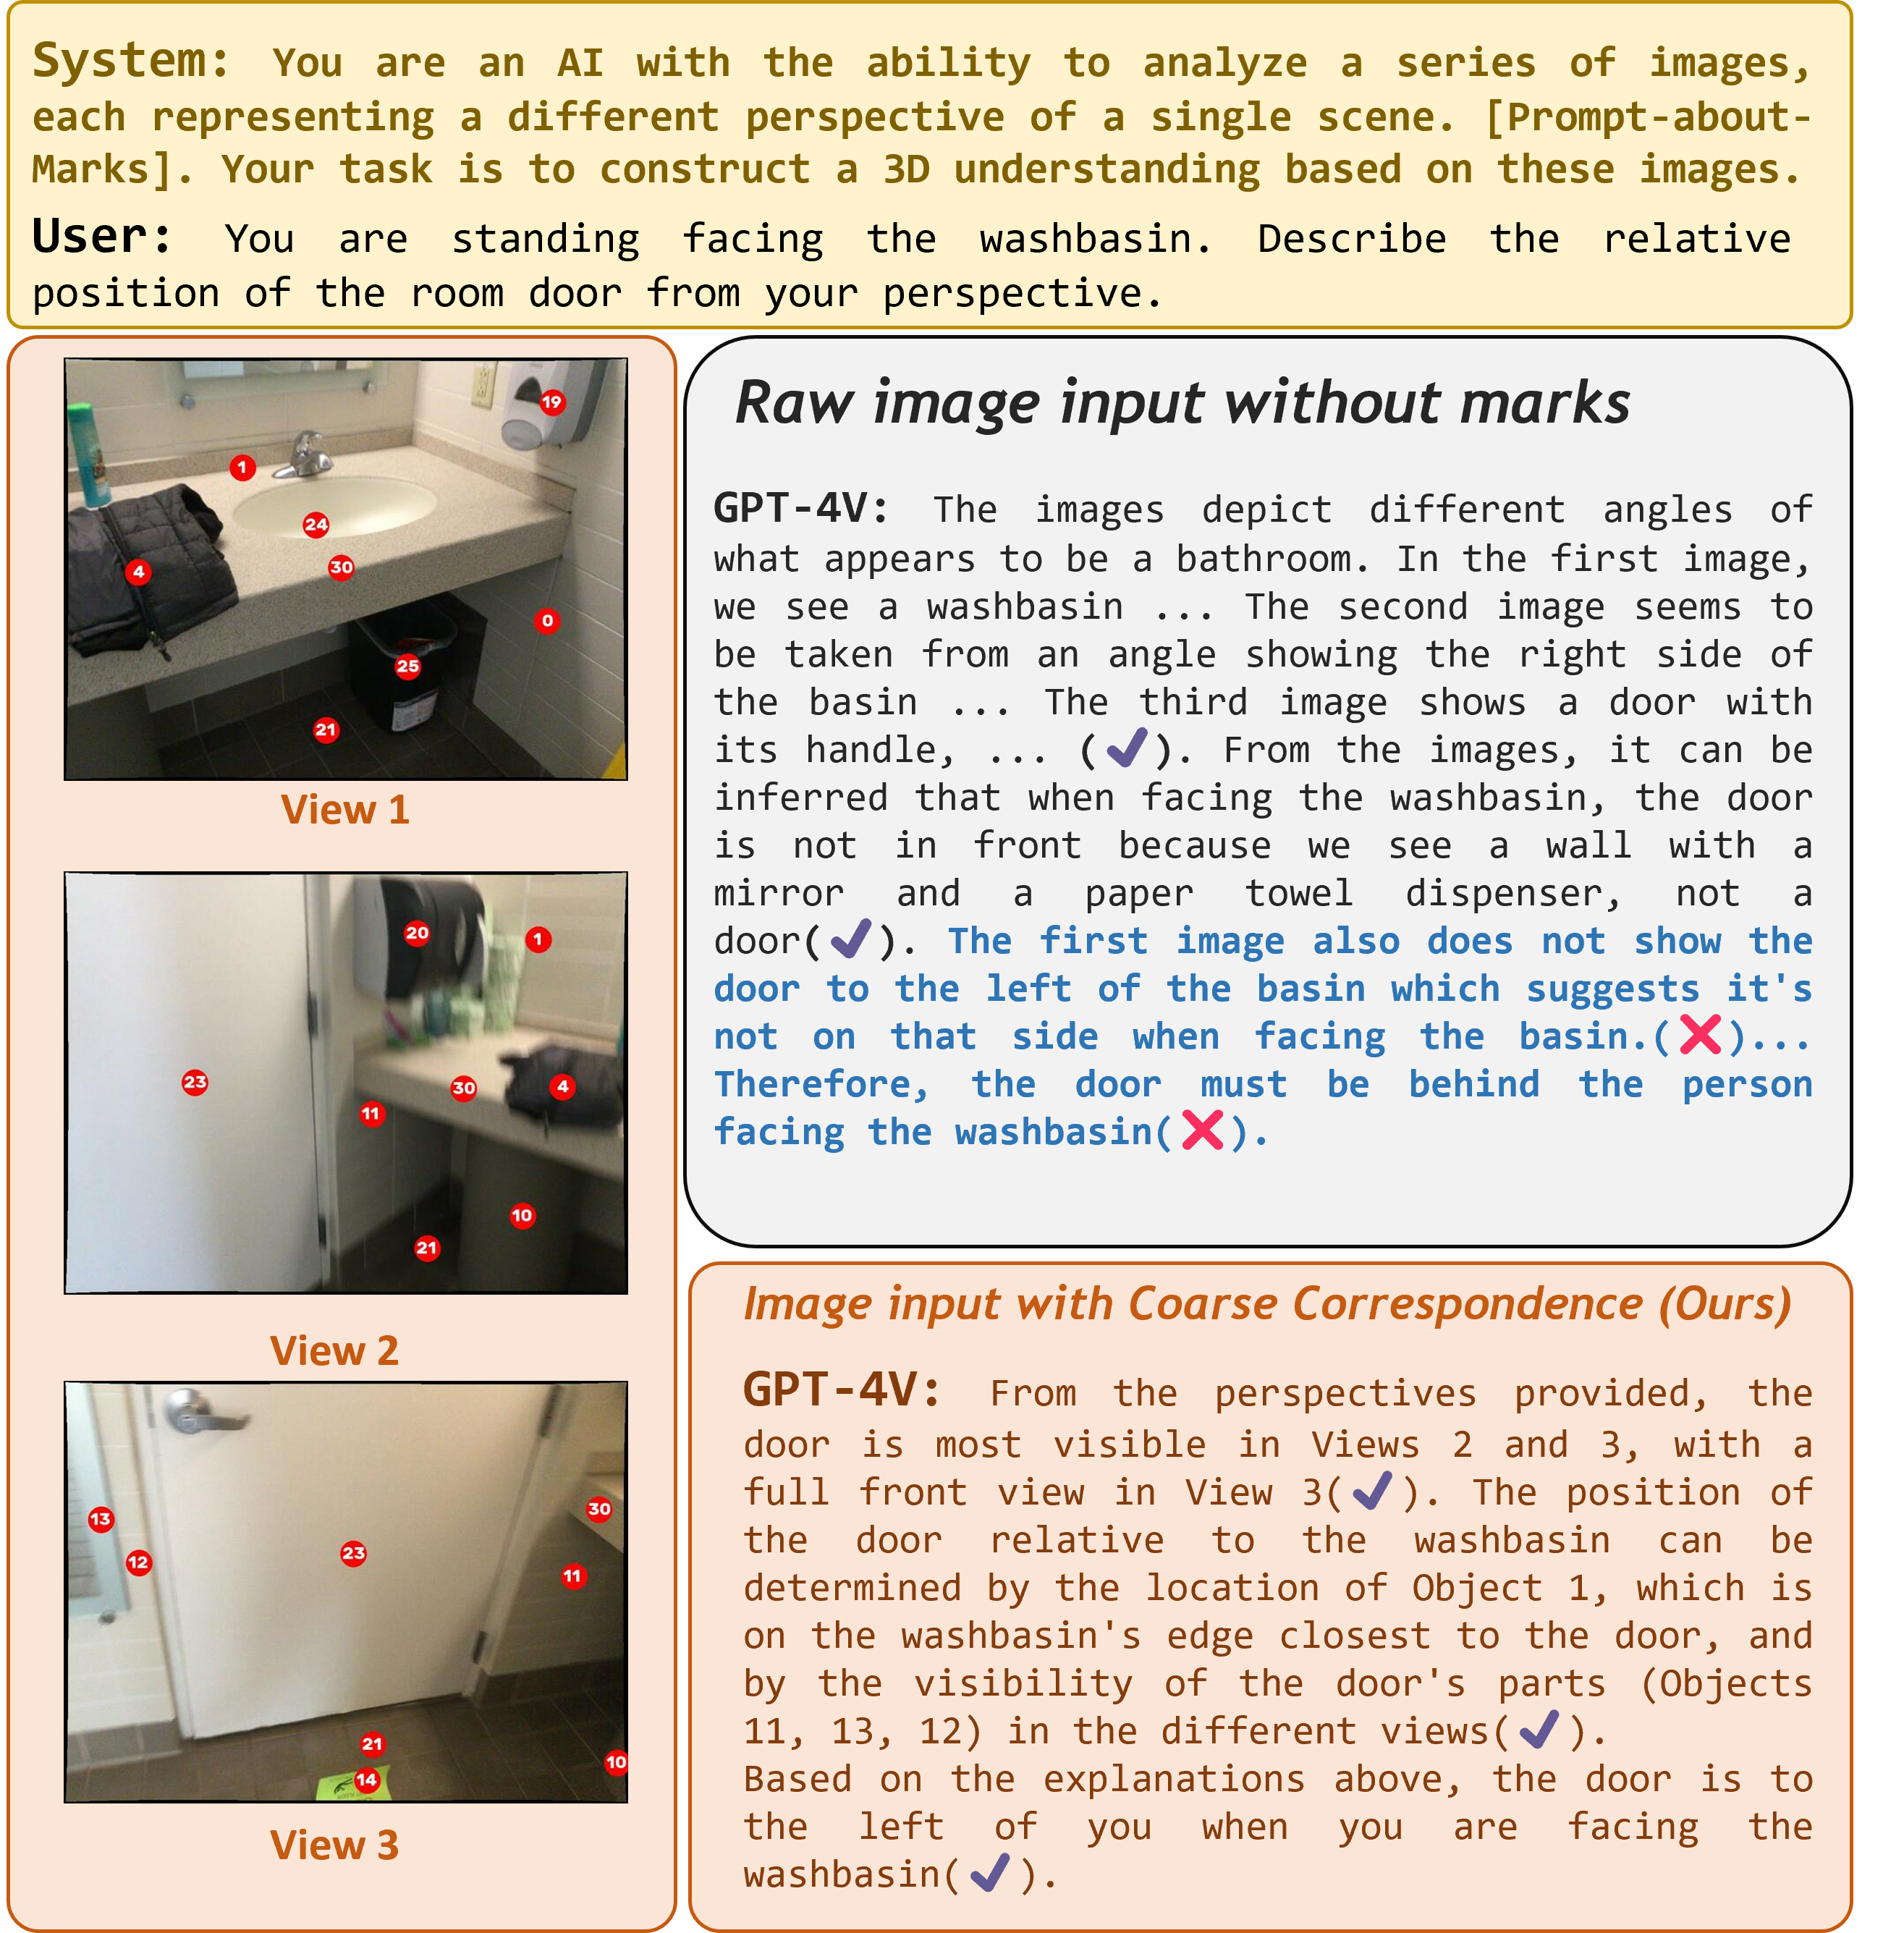}
        \caption{\textbf{Task: Relative Location Modeling.} From View 1 \& 2 we can tell that the room door is on the left-hand-side when facing the washbasin. Only with the help of the Coarse Correspondence can GPT-4V understand relative location between objects appear in different views across a single 3D scene.}
        \label{fig:relative_location}
    \end{subfigure}
    \caption{Two complicated tasks, i.e. Duplicate Objects Counting and Relative Location Modeling are chosen to demonstrate our method. Zoom in for better view.}
    \label{fig:two_example}
\end{figure}

To further demonstrate the effectiveness of our proposed Coarse Correspondence under sparse image input,
we defined two challenging tasks and one qualitative case study for each task.

The results of these case studies are shown in Fig. \ref{fig:two_example}.
Detailed illustration of the results are provided in the figure captions.
The first case study is about the task of Duplicate Objects Counting,
where the model needs to count the number of objects in a 3D scene.
Only equipped with coarse correspondence can GPT-4V get a comprehensive understanding of the 3D scene, excludes the duplicate objects, and give the right answer.The second case study is about the task of Relative Location Modeling,
where the model needs to understand the relative location of objects in a 3D scene.
It is obvious that without the correspondence markers, GPT-4V fails to response from 3D perspective with only raw 2D images.These case studies demonstrate that our proposed Coarse Correspondence can elicit
MLLMs in understanding 3D scenes from sparse image inputs.

\begin{figure}[]
    \centering
    \includegraphics[width=0.95\linewidth]{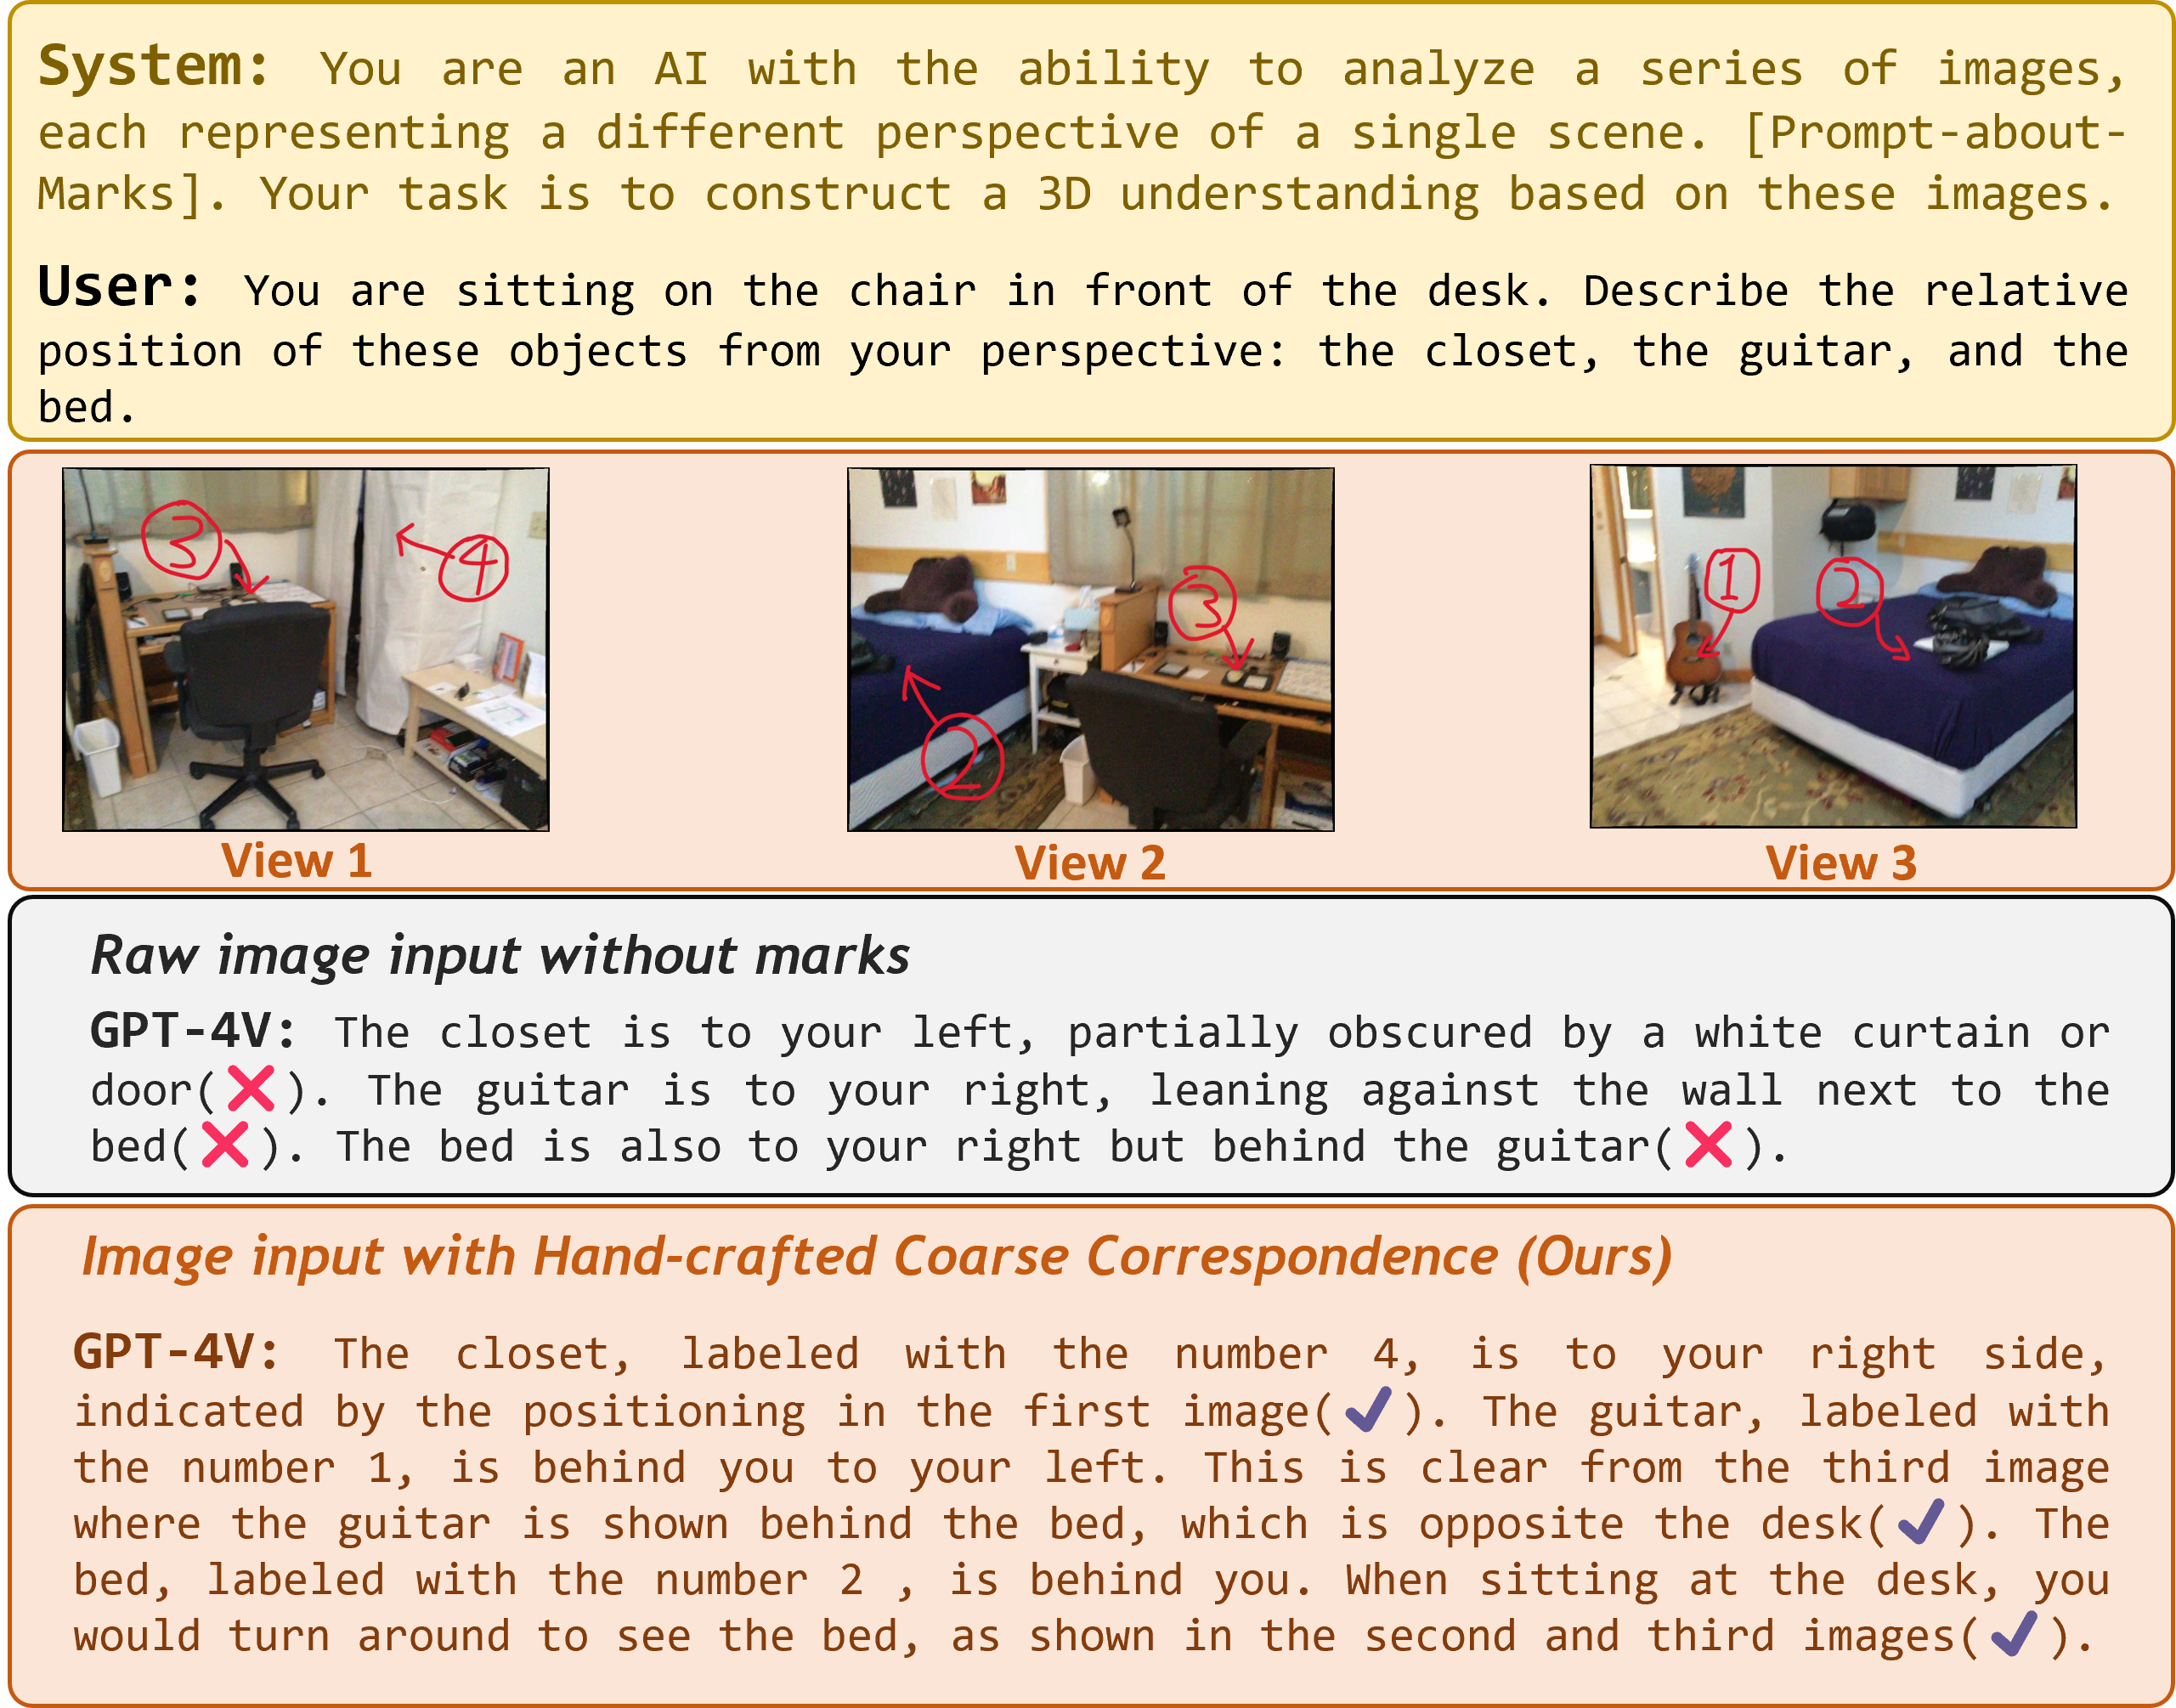}
    \caption{\textbf{Hand-crafted coarse correspondence label.} Coarse correspondence can still help the spatial understanding when using hand-crafted visual prompting.}
    \label{fig:handcrafted_prompt}
\end{figure}

\section{User-Friendly Interactions}
We also prove that our Coarse Correspondence method works well with 
hand-crafted correspondence marks as shown in ~\Cref{fig:handcrafted_prompt}. 
This demonstrates that our method is highly user-friendly for utilizing proprietary multimodal language models, such as GPT-4O, in web interfaces. Users can easily complete prompts by marking correspondence relationships on images. Moreover, the marks can be diverse and flexible. This also proves the robustness of our method, as the marks are style-agnostic, as long as they convey the visual correspondence knowledge.
